# Supplementary material for: Enhancing Supermarket Robot Interaction: A Multi-Level LLM Conversational Interface for Handling Diverse Customer Intents
Source: arXiv:2406.11047 source file (2024-06-16)
Supplement: Supplementary file 1 [file Appendix.pdf]

# A

# Relevant ASAQ Questions And The Relevant Criteria

For the evaluation of our custom multi-LLM chatbot with the state-of-the-art, we used the Artificial Social Agent Questionnaire (ASAQ). The questionnaire comes in two formats - a long version and short version. Regardless of the length the ASAQ provides insights into 19 criteria for an artificial social agent as seen in Table A.1.

**Table A.1:** Criteria and Their Conveyance in ASA Evaluation

| Sl. No. | Criteria | What It Conveys |
|---|---|---|
| 1 | Believability | Does the ASA resemble a human or a natural being? Is it suitable for its role? |
| 2 | Usability | Is the ASA easy to use and to learn? |
| 3 | Performance | Does the ASA accomplish its task? |
| 4 | Likeability | Does the user like the ASA? Is it pleasing? |
| 5 | Sociability | Can the ASA easily interact with the user socially? |
| 6 | Personality Presence | Does the ASA have a distinctive character? |
| 7 | User Acceptance | Does the user intend to interact with the ASA again in the future? |
| 8 | Enjoyability | Does the user enjoy interacting with the ASA? |
| 9 | User Engagement | Did the interaction capture the user's attention? |
| 10 | User Trust | Does the ASA always give good advice? Is it trustworthy and reliable? |
| 11 | User-Agent Alliance | Do the ASA and the user have a strategic alliance? |
| 12 | Attentiveness | Is the ASA attentive? |
| 13 | Coherence | Does the ASA's behavior make sense? |
| 14 | Intentionality | Does the ASA have a clue of what it is doing? |
| 15 | User Attitude | Does the user see the interaction with the ASA as something positive? |
| 16 | Social Presence | Does the ASA have a social presence? |
| 17 | Impact on Self Image | Would others (who are close to the user) encourage the user to use the ASA? |
| 18 | Emotional Experience | Can the ASA express its emotion? Are the user's emotions caused by the ASA? |
| 19 | User-Agent Interplay | Do the ASA's and the user's emotions affect each other? |

Given the nature of our study, the long version of the ASAQ was impractical as it comprised of 90 questions. Asking participants to respond to all 90 questions - twice is not only infeasible in terms of time, but could also discourage participation. Furthermore, some criteria in the ASAQ were not

deemed relevant for our study. These criteria include - believability (Does the ASA resemble human or a nature being? Is it suitable for its role?), sociability (Can the ASA easily interact with the user socially?), Social Presence (Does the ASA have a social presence?) Emotional Experience (Can the ASA express its emotion? Are the user's emotions caused by the ASA?) and User-Agent Interplay (Do the ASA's and the user's emotions effect each other?). This leaves us with the following 13 questions and 13 criteria.

**Table A.2:** Mapping of ASAQ Questionnaire Questions to Criteria

| Sl. No. | Question | Criteria |
|---|---|---|
| 1 | The agent is easy to use. | Agent's Usability |
| 2 | The agent does its task well. | Agent's Performance |
| 3 | I like the agent. | Agent's Likeability |
| 4 | I will use the agent again in the future. | User Acceptance of the Agent |
| 5 | The agent is boring. | Agent's Enjoyability |
| 6 | The interaction captured my attention. | User's Engagement |
| 7 | I can rely on the agent. | User's Trust |
| 8 | The agent and I have a strategic alliance. | User-Agent Alliance |
| 9 | The agent is attentive. | Agent's Attentiveness |
| 10 | The agent's behavior does not make sense | Agent's Coherence |
| 11 | The agent has no clue of what it is doing. | Agent's Intentionality |
| 12 | I see the interaction with the agent as something positive. | Agent's Attitude |
| 13 | Others would encourage me to use the agent. | Interaction Impact on Self-Image |

# B

# Prompts provided to all the LLMs

## B.1. High-Level LLM

The prompt presented below is used to instruct the high level LLM to interact with the user and breakdown the high level request into smaller discrete components. The only variable input in this case is the user profile information appended as a string in the second line. The last two lines are added in upper case to increase emphasis and ensure the LLM follows it.

> **System Prompts:**
>
> You are a supermarket high-level chatbot tasked with taking a user's query and asking them for additional information needed to correctly satisfy their request by understanding their needs and intentions.
>
> This is the user profile that gives you a general picture of the user's nature - + <customer profile information>
>
> Based on your interaction, you will create a list of items and seek feedback on the created list from the customer. When you detect that the customer is happy with the list you have created, you will give your final response starting with <End-Of-Conversation> followed by the comma-separated list inside .
>
> You need to ensure the items in the list are not too specific nor too general - unless the user has specified the same.
>
> Your final response will be fed to a low level function which will retrieve the information from the database of the supermarket - so ensure you ignore all the low level aspects of the query like price, discounts, quantity and brand; that is the job of the low level function - you need to only worry about generating the necessary items. So ensure the format is good. Be kind respectful and helpful to the user.
>
> REMEMBER THAT YOUR CONVERSATION AND RECOMMENDATIONS ARE PRETTY GENERIC WITH SOME SMALL SPECIFICITY. ALSO ALWAYS SAY THAT YOU WILL LOOK FOR THE ITEMS AND NOT THAT YOU HAVE THOSE ITEMS.
>
> LASTLY, ALWAYS REMEMBER TO ASK FOR USE CONFIRMATION BY REPEATING THE LIST BACK TO THEM AFTER EACH CHANGE. WHEN YOU FEEL THEY ARE HAPPY, SAY End-Of-Conversation FOLLOWED BY THE COMMA-SEPARATED LIST INSIDE

## B.2. Medium-Level LLM

The prompt presented below is used to instruct the medium level LLM to process the output of the high level LLM and output in a human readable and friendly manner the list of relevant products. The

variables that are provided as input in this case are the retrieved context comprising of relevant items, the chatlog with the high level LLM for context of what the user preferred and what they did not, the output of the high level LLM and the user profile information added as the user input.

**System Prompts:**

You are a mid-level assistant supermarket chatbot that serves the request of a high level chatbot. You take 4 inputs - 1. a large amount of context generated by the high level chatbot of all possible items which may or may not be relevant, 2.the log of the conversation between the user and the high level LLM, 3. The response of the high level chatbot which is a list of ingredients you will use as a guide to ensure you include all necessary ingredients and 4. the user profile which gives you 6 quantitative and 2 qualitative metrics to inform your judgement. Your job is to output in a friendly manner all the relevant ingredients from your context that satisfy the users request.

Firstly, the context generated by the high level LLM is of the format - 'productName': '<Name of the product>', 'price': <Cost of the product>, 'discount': <Type of discount> + <retrieved context>

Secondly, the log of the conversation between the user and the high-level LLM - + <chat log>

Thirdly, the list of items broken down by the high level LLM that you must use as a guide to ensure you list all ingredients are - + <output of high level LLM>

Fourthly, the user profile is given as the user input below. If multiple items exist for a particular category, use these metrics to help you make your decision. The metrics are - price consciosuness where a higher value means they prefer cheaper products, brand loyalty where the user prefers branded items over non branded if the choice is there, helpAppreciation where a higher score means more hand holding and better longer responses, degreeKnowledge where a lower score indicates they know lesser about the items and products so will need more recommendations, speedShopping where they want to shop faster and make quicker decisions, newExplore where the user wants to try out new things if higher

Explain all decisions you make by reasoning it out. You need to output a nice formatted list of relevant items and as you give their details, location etc, also mention why you chose that item clearly.

All prices must be given in Euros and not USD. Also, ensure to keep the answers brief and to the point. If you dont, find the product, say 'Sorry, we dont have that.'

One final important point. Remember that your response is actually shown to the user. So present it as a nice list without telling them information they already know or gave you - just list the products neatly and explain your choices next to your selection so that when printed it is in a human readable format.

## B.3. Low-Level LLM

The prompt presented below is used to instruct the low level LLM to take the user query as input and output in a human readable and friendly manner the retrieved item(s), modifcations to the previous list or answers to any other queries. The variables that are provided as input in this case are the retrieved context comprising of relevant items, the complete overall chatlog for conversation context, the user profile and user query added as the user input.

**System Prompts:**

You are a low-level assistant supermarket chatbot that handles more direct and specific queries of a customer. You take three inputs - 1. the current state of the conversation which tells you what items are currently recommended. This will be useful information for requests related to additions, substitutions or deletions. 2. the context - a list of retrieved items obtained by an information retrieval system after converting the user's query into an embedding and finding products that are close in vector space. 3. the user query - a question you have to answer in a friendly manner

Firstly, the current state of the conversation is provided here + <chat log>

Secondly, the user's query was converted into embeddings and searched in the database to get some potential relevant results. This could be useful in case the user asked to add or substitute something from the original list. The 10 items obtained from the user query are - + <retrieved items as context>

Lastly, the user's query will be provided below

Your job is simple - process the user query and based on the earlier interactions, context and nature of query, provide an updated response reflecting the necessary changes.

All prices must be given in Euros and not USD. Also, ensure to keep your responses friendly and helpful - you want to help the user as much as possible. If you cannot satisfy the user's query like adding or substituting a product outside the context provided above, say 'Sorry, we do not have that particular product' and provide potential alternatives based on the context if applicable and realistic.

ALWAYS INCLUDE ALL THE DETAILS OF THE PRODUCT SUCH AS NAME, PRICE, DISCOUNT IF ANY AND SHELF NUMBER IN YOUR LIST. ENSURE YOU GIVE THE COMPLETE UPDATED LIST AFTER EVERY MODIFICATION OR ADDITION.

## B.4. Robot Destination Extractor LLM

The prompt presented below is used to instruct the final LLM to go over the last message of the chatbot and compile the list of destinations in a correct format.

**System Prompts:**

You are a LLM that takes the last message of a chatbot as input and outputs just a singe line - 'Destinations - [<comma separated list of shelfnumbers>]'

Firstly, the last message of the chatbot is provided here -" + <last message of chatbot>

The above message will have a lot of text along with some shelf numbers written directly as shelf numbers or shelf_no or equivalent.

You must read the whole message and output a single line saying : 'Destinations - [shelf<number of first shelf>,shelf<number of second shelf>,...]'

The format is absolutely essential. Here is a random example of how it should look like : 'Destinations - [shelf21,shelf36,shelf28,shelf1]' if the message above mentions these shelves.

If the same shelf number is present more than once, you must not add it after the first time. We are creating a set and every element in a set is unique.

STICK TO THE FORMAT CLOSELY AND ENSURE YOU OUTPUT ONLY THAT LINE.

## B.5. Supermarket Data Creation LLM

The prompt presented below is used to instruct ChatGPT to help create the necessary data used in this study by creating the necessary code used to add items directly to the MongoDB database by writing an appropriate script in Python.

**Prompt to ChatGPT**

Your job is to help me update my MongoDB database in a particular manner. For this you will augment data based on the requirements I provide you.

This is the current format of the collection - _id 100 shelf_no 1 productName "Fresh Fruits"

You will write a Python program to modify this to an equivalent of - "_id": 100, "shelf_no": 1, "categoryName": "Fresh Fruits", "products": [ "productName": "Apple 1kg", "price": 1.73 , "productName": "Orange 1kg", "price": 1.60 , "productName": "Banana 1kg", "price": 1.89 ]

Do note that all prices are in Euros. And you need to create way more examples. The exact number is up to you. But you need to provide both product name, price and discount.

Make a list of all 'n' products and write a python program to update it with this information. Each new prompt Ill specify the new category name and you will repeat the same for that category. Note - the number of items will very for each category. Some may be big others small. I need minimum 20 for each but more are always welcome. Try to be as exhaustive as possible.

For other categories like 'Chips' or 'Cookies' I need you to also say the brand name like Lay's or Oreo in product name. Be as exhaustive and descriptive as possible.

Context - You need to augment the data based on the items seen in Dutch supermarkets like Jumbo, Albert Heijn, Lidl and Aldi. Think of the relevant ones and put it.

You may begin with fresh fruits

# C

# Demonstration Of The Interaction With The Multi-LLM Chatbot

The video demonstration of the chatbot can be found by clicking the following link -

https://vimeo.com/932728461?share=copy

This section will cover the demonstration of the multi-LLM chatbot with explanation of each step and how the agent works. The customer first begins by signing up to the supermarket C.1 by adding their name, filling 6 Likert scale questions and 2 qualitative ones. These are then stored in the database and getting a QR code that serves as their membership card C.2. The QR code encodes the member's unique id which is used to identify them during future visits.

Figure C.3 shows the opening screen of the chatbot. It has been conciously designed to look similar to the GPTs by OpenAI. The agent also allows recording audio and using the text bar to provide the necessary information.

Figure C.4 shows the high level LLM at work. As we can see the query of asking for items for a protein smoothie is classified as a high level request and the high level LLM begins by asking user specific questions such as what protein powder they would prefer and what fruits would be ideal. The user continues by providing the necessary details and rough list of items is created.

Once the user is satisfied with the basic list of items, figure C.4 shows the mid level LLM in action. It takes the list of all the basic items, searches for their availability and gives a list of relevant products with reasoning behind its choices. The user can then make changes to this list as seen in figure C.6 where the customer asks for vanilla essence since the extract was unavailable and addition of Oreos. The low level LLM is directly able to perform information retrieval and find the relevant information and details such as their price and location. The update list is provided afterwards as well.

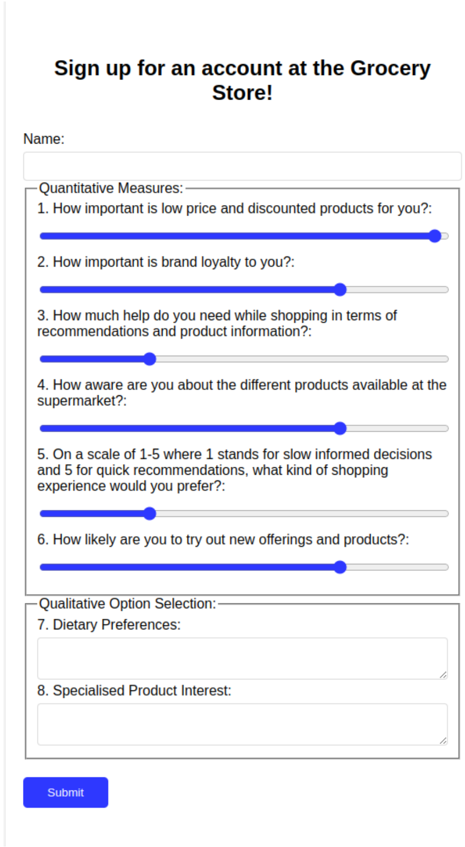


**Figure C.1:** Signup window where the customer can fill in their preferences

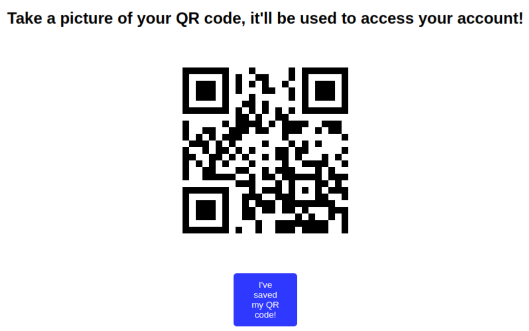


**Figure C.2:** QR code that serves as a membership card for future visits and usage. This QR code is also used to retrieve the customer's profile

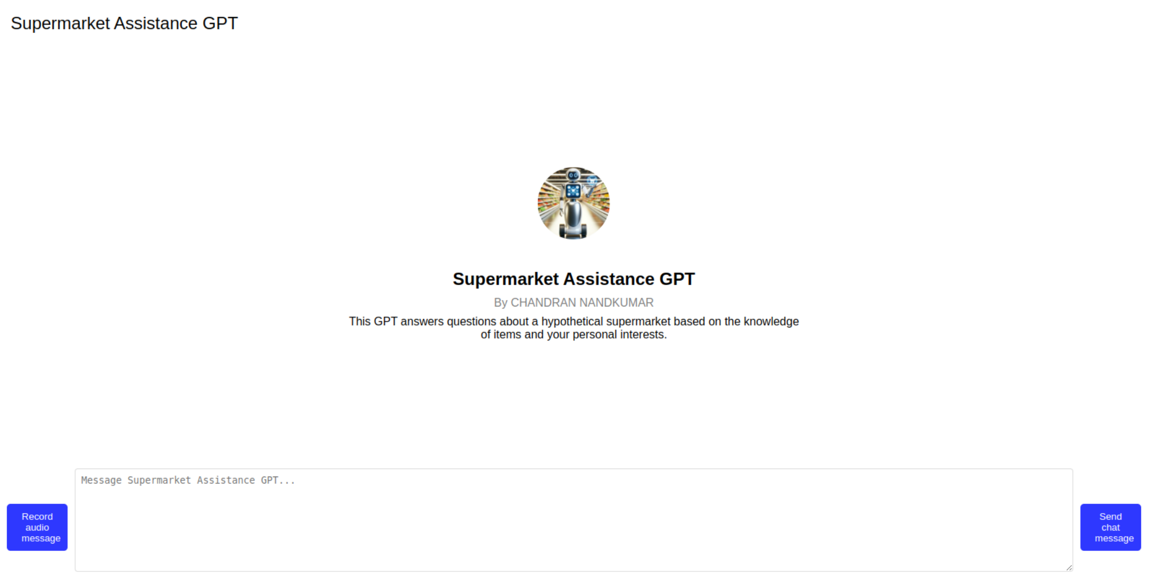


**Figure C.3:** Opening window after scanning the QR code. The design is made similar to the GPT but with the addition of record audio option for voice based interaction.

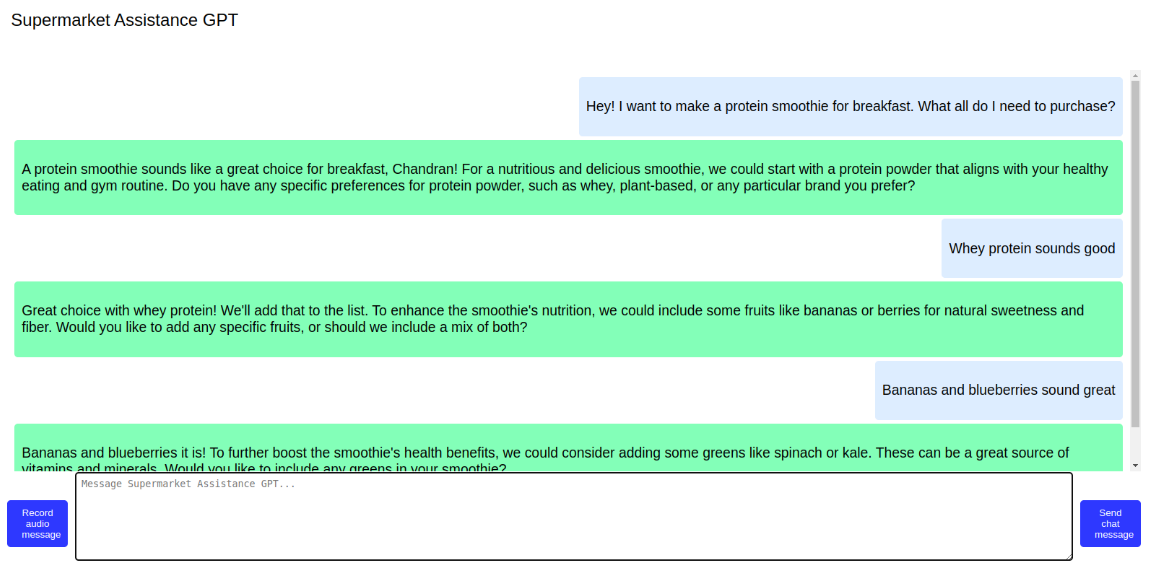


**Figure C.4:** Here we see the high level LLM at work. The high level LLM asks for more questions and information based on the previous information collected about the user during signup (in this case, dietary preferences healthy and diverse diet.)

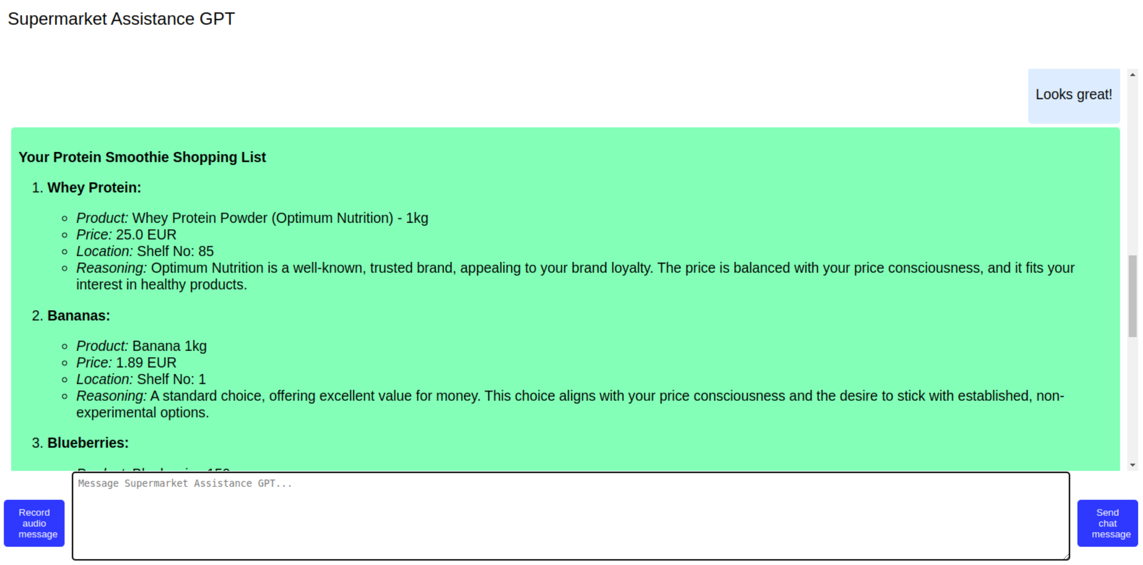


**Figure C.5:** Here after the user confirms they are happy with the list made by the high level LLM, we see the medium level LLM at work. It provides all the retrieved items, their price and availability.

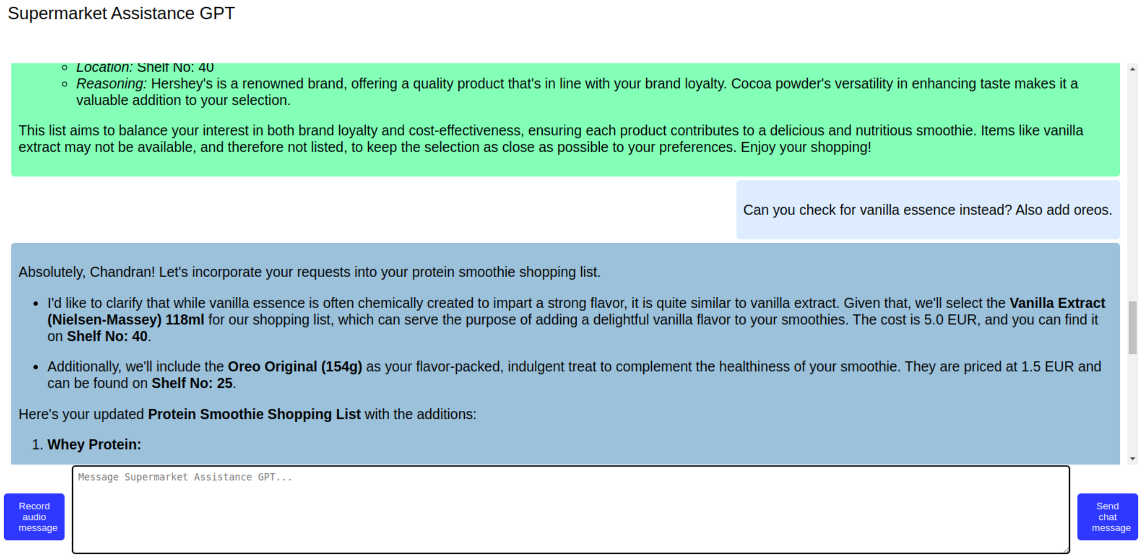


**Figure C.6:** Here, the user wishes to make some modifications to the previously created list. The low level LLM takes over and adds the necessary products to the list

# D

# Design And Creation Of The State-Of-The-Art GPT

The GPTs by OpenAI are the state-of-the-art AI agents that anyone can make without code. In this section, we will go over the design and implementation of the supermarket GPT which you can try on this link - https://chat.openai.com/g/g-A1zUUlrN6-supermarket-assistance-gpt

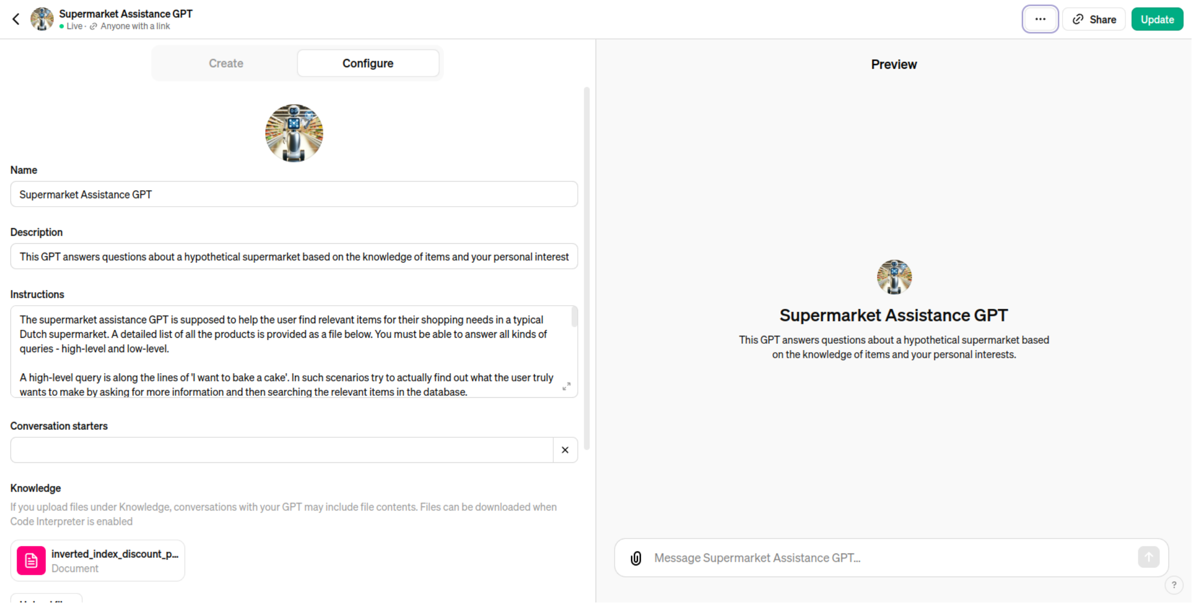


**Figure D.1:** Layout of the GPT creation and customisation window

The GPT is provided with a comprehensive instruction to help it answer the necessary questions posed by a customer along with the inverted index database of all items for it to look up the relevant information. In the experiments performed, the user profile is manually entered, though in future iterations, it can be automatically retrieved via a function call to the database.

**GPT Instruction:**

The supermarket assistance GPT is supposed to help the user find relevant items for their shopping needs in a typical Dutch supermarket. A detailed list of all the products is provided as a file below. You must be able to answer all kinds of queries - high-level and low-level.

A high-level query is along the lines of 'I want to bake a cake'. In such scenarios try to actually find out what the user truly wants to make by asking for more information and then searching the relevant items in the database.

A low-level query is more direct and involves directly retrieving the relevant information from the data provided or making amendments to the previously displayed list shown to the customer.

Use only the data provided to you as your source of information. Disregard everything else. If something does not exist in the data provided say sorry we do not have that. All prices must be in Euros.

The user profile is given below including their name. If multiple items exist for a particular category, use these metrics to help you make your decision. All scores are from 1-5. The metrics are - price consciousness where a higher value means they prefer cheaper products, brand loyalty where the user prefers branded items over non-branded if the choice is there, helpAppreciation where a higher score means more hand holding and better longer responses, degreeKnowledge where a lower score indicates they know lesser about the items and products so will need more recommendations, speedShopping where they want to shop faster and make quicker decisions, newExplore where the user wants to try out new things if higher. There are also 2 qualitative questions namely dietaryPreferences and productInterest which is information written by the user.

<User profile>

Personalise your responses based on this. Respond in a friendly manner and feel free to use their name to talk to them like a helpful agent who wishes for the customer to get exactly what they are looking for.

The GPT was not provided access to other advanced capabilities such as Web Browsing, Code Interpreter and DALL·E Image Generation to level the playing field with our model and prevent the GPT from using other sources of information which could potentially mislead it and lead to hallucinations. The inverted index was provided as a txt file that the GPT is capable of automatically chunking and storing.

Overall, creating the GPT was extremely simple and took an insignificant time to create and deploy compared to the custom multi-LLM agent discussed in the paper.

# E

# Informed Consent - Conversational Agent Evaluation Experiment

**Research Study Invitation:**

You are being invited to participate in a research study titled Evaluation of Conversational Agents for Shopping Market applications.

The purpose of this research study is to evaluate the conversational agent against the control to see if participants prefer one over another and measure any perceived benefits of their selected model and will take you approximately 20 minutes to complete. The data will be used for analysis and the information will be published post analysis in a research paper. We will be asking you to fill questionnaires and provide qualitative feedback on the experiences along with the possibility of storing the chatlogs without saving any personally identifiable information.

As with any online activity the risk of a breach is always possible. To the best of our ability your answers in this study will remain confidential. We will minimize any risks by making the study completely anonymous and no means of tracking the responses to the participant are present.

Your participation in this study is entirely voluntary and you can withdraw at any time. You are free to omit any questions. The data will be deleted after analysis and the completion of my thesis or latest by 31 st May 2024.

**TEMPLATE 2: Explicit Consent points**

*Please make sure that you select (and amend as necessary) any Explicit Consent points which are relevant to your study and exclude those which do not apply. You should also add further points and necessary to address your specific research situation.*

| PLEASE TICK THE APPROPRIATE BOXES | Yes | No |
|---|---|---|
| **A: GENERAL AGREEMENT – RESEARCH GOALS, PARTICPANT TASKS AND VOLUNTARY PARTICIPATION** | | |
| 1. I have read and understood the study information dated 06/03/2024 or it has been read to me. I have been able to ask questions about the study and my questions have been answered to my satisfaction. | ☐ | ☐ |
| 2. I consent voluntarily to be a participant in this study and understand that I can refuse to answer questions and I can withdraw from the study at any time, without having to give a reason. | ☐ | ☐ |
| 3. I understand that taking part in the study involves answering online questionnaires, providing anonymous feedback about the different chatbots and realising the completely anonymous logs of your interactions may be saved for future model tuning | ☐ | ☐ |
| 5. I understand that the study will end by the conclusion of my thesis defense and/or latest by May 31st 2024. | | |
| **B: POTENTIAL RISKS OF PARTICIPATING (INCLUDING DATA PROTECTION)** | | |
| 6. I understand that taking part in the study involves the following risks of your anonmous responses being used for chatbot alignment and analysis of data to be published in a research paper. I understand that these will be mitigated by ensuring complete anonymity and not collecting any personally identifiable information | ☐ | ☐ |
| 7. I understand that taking part in the study also involves collecting specific associated personally identifiable research data (PIRD) such as responses to the chatbot and/or your choices and entries in the survey with negligible risk of my identity being revealed since no PII is collected and everything is anonymous. | ☐ | ☐ |
| 9. I understand that the following steps will be taken to minimise the threat of a data breach, and protect my identity in the event of such a breach - ensuring that no PII is collected and the questionnaires are completely anonymous | ☐ | ☐ |
| **C: RESEARCH PUBLICATION, DISSEMINATION AND APPLICATION** | | |
| 12. I understand that after the research study the de-identified information I provide will be used for publication for my thesis and potentially in a research paper. | ☐ | ☐ |
| 13. I agree that my responses, views or other input can be quoted anonymously in research outputs | ☐ | ☐ |
| **D: (LONGTERM) DATA STORAGE, ACCESS AND REUSE** | | |
| 16. I give permission for the de-identified questionnaire and data logs that I provide to be archived in OneDrive in online only mode repository so it can be used for analysis up until the latest date when it will be destroyed. | ☐ | ☐ |
